# Supplementary material for: Deep Coarse-grained Potentials via Relative Entropy Minimization
Source: arXiv:2208.10330 ancillary file (2023-01-03)
Supplement: Supplementary file 1 [file Supplement.pdf]

# Deep Coarse-grained Potentials via Relative Entropy Minimization: Supporting Information

Stephan Thaler[1], Maximilian Stupp[1], and Julija Zavadlav[1,2]

[1]*Professorship of Multiscale Modeling of Fluid Materials, Department of Engineering Physics and Computation, TUM School of Engineering and Design, Technical University of Munich, Germany*
[2]*Munich Data Science Institute & Munich Institute for Integrated Materials, Energy and Process Engineering, Technical University of Munich, Germany*

## Contents

**Supplementary Methods** 1
1. Liquid Water . . . . . . . . . . 1
2. Alanine Dipeptide . . . . . . . . . . 1

**Supplementary Figures** 2

**Supplementary References** 7

# Supplementary Methods

We train all models via the Adam optimizer [1] with default parameters, except for the learning rate. We decay the initial learning rate $\eta_0$ by an exponential decay schedule such that the $\eta_0$ is reduced by a factor 0.01 at the end of the training. For force matching (FM), we set $\eta_0 = 0.001$, the default value of the Adam optimizer. For relative entropy (RE) minimization, we choose a larger step size $\eta_0 = 0.003$ as the model needs to converge within a significantly smaller number of updates. All CG simulations are run in JAX, M.D. [2] on a single Nvidia RTX 3090 GPU.

## 1. Liquid Water

To generate the atomistic (AT) reference data, we run a LAMMPS [3] simulation with time step 2 fs. Initially, the box size is set by a 1 ns NPT simulation with target pressure of 1 atm. After equilibrating the system for 1 ns in the NVT ensemble, we generate the 10 ns data trajectory.

All CG simulations use a Nose-Hoover [4] thermostat with a chain length of 3, 3 Suzuki-Yoshida steps and a coupling time of 200 fs. We subsample generated trajectories such that a state is retained every 0.1 ps.

For RE training, we approximate the AT average (first term) in eq. 8 via an average over random batches consisting of 700 states from the AT data set. This reduces the overhead from averaging over the whole AT data set significantly. Given that we average over the same number of states as generated by the CG MD simulation, we do not expect a meaningful increase in the statistical error of the computed gradient. Increasing the number of states considered in both averages offers a systematic way to decrease the statistical noise, if necessary.

We discretize the radial distribution function (RDF) with 300 bins, the triplet correlation function (TCF) with 50 bins in each direction and the ADF with 150 bins. For the ADF, we select a triplet cut-off value of 0.318 nm, which is consistent with experimental evaluations [5].

## 2. Alanin Dipeptide

We generate the AT reference trajectory via a NVT simulation in GROMACS [6] using the AMBER03 [7] force field, which resolves hydrogen atoms. The protein is solvated in TIP3P water. The simulation employs a veloctiy-rescaling thermostat [8] with a time constant $\tau = 0.1$ ps and a time step of 2 fs. We equilibrate the system for 1 ns

in the NVT ensemble and 1 ns in the NPT ensemble with a barostat pressure of 1 bar, before generating the 100 ns reference trajectory in the NVT ensemble.

All CG simulations use a Langevin thermostat with $\gamma = 100\ \mathrm{ps}^{-1}$ and a time step $\Delta t = 2$ fs. Generated trajectories are subsampled such that a state is retained every 0.2 ps. We discretize the $\phi$ and $\psi$ density histograms and free energy surfaces via 60 bins each. The data set variation study in fig. 7 follows the default training scheme detailed above with 100 training epochs, except for the small 10 ns data set, which we train for 1000 epochs to have the same number of updates as with the 100 ns reference data set. For the convergence analysis in fig. 8, we increase the learning rate decay factor to 0.1 due to the even smaller number of updates. We note that in practice, a smaller initial learning rate than $\eta_0 = 0.003$ might be appropriate to avoid changing the FM potential beyond the necessary.

# Supplementary Figures

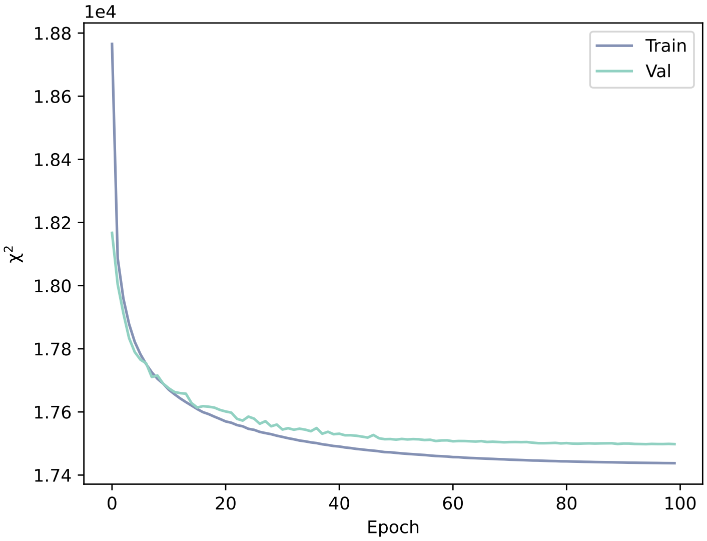


Figure 1: Liquid water loss curves. Per-epoch training and validation loss $\chi^2$ for force matching training of the liquid water model.

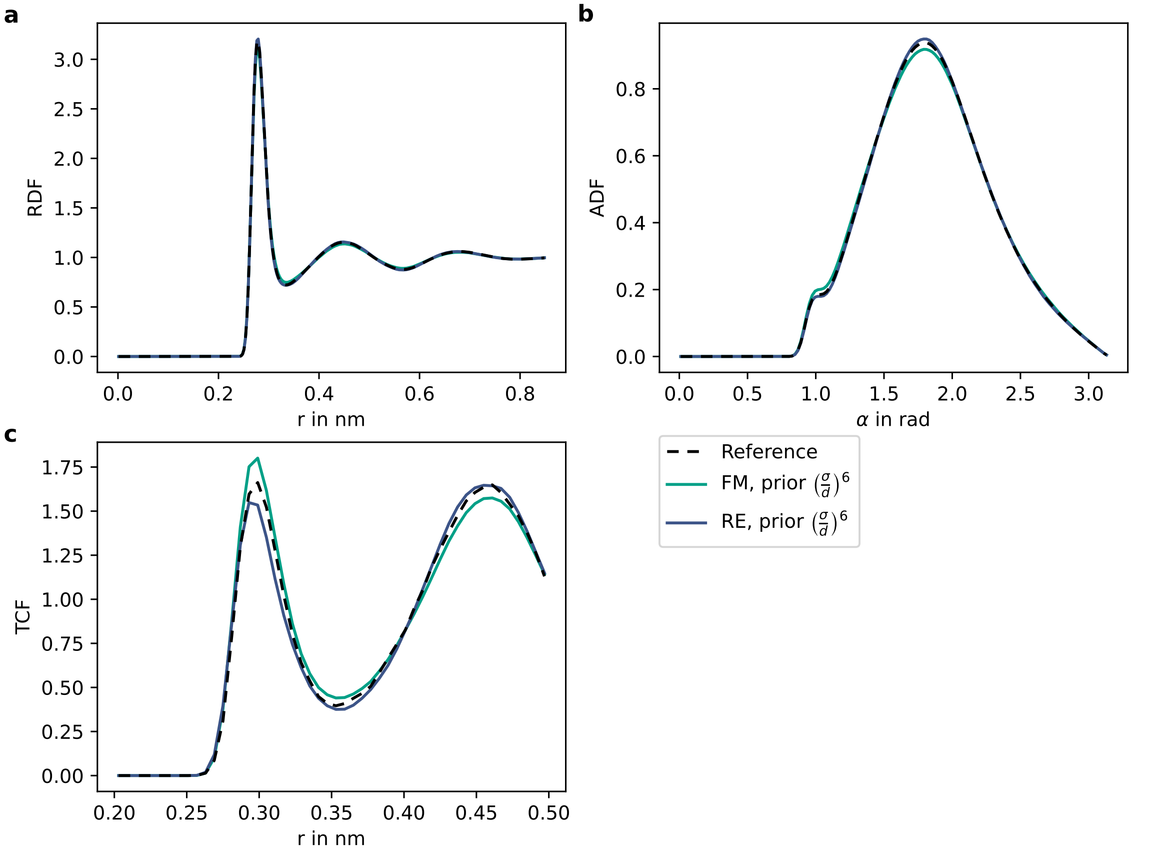


Figure 2: Liquid water prior variation. Resulting (**a**) radial (RDF) and (**b**) angular distribution function (ADF) [5] as well as (**c**) equilateral triplet correlation function (TCF) [9, 10] of models with a prior exponent of 6 trained via force matching (FM) and relative entropy (RE) minimization compared to the atomistic reference.

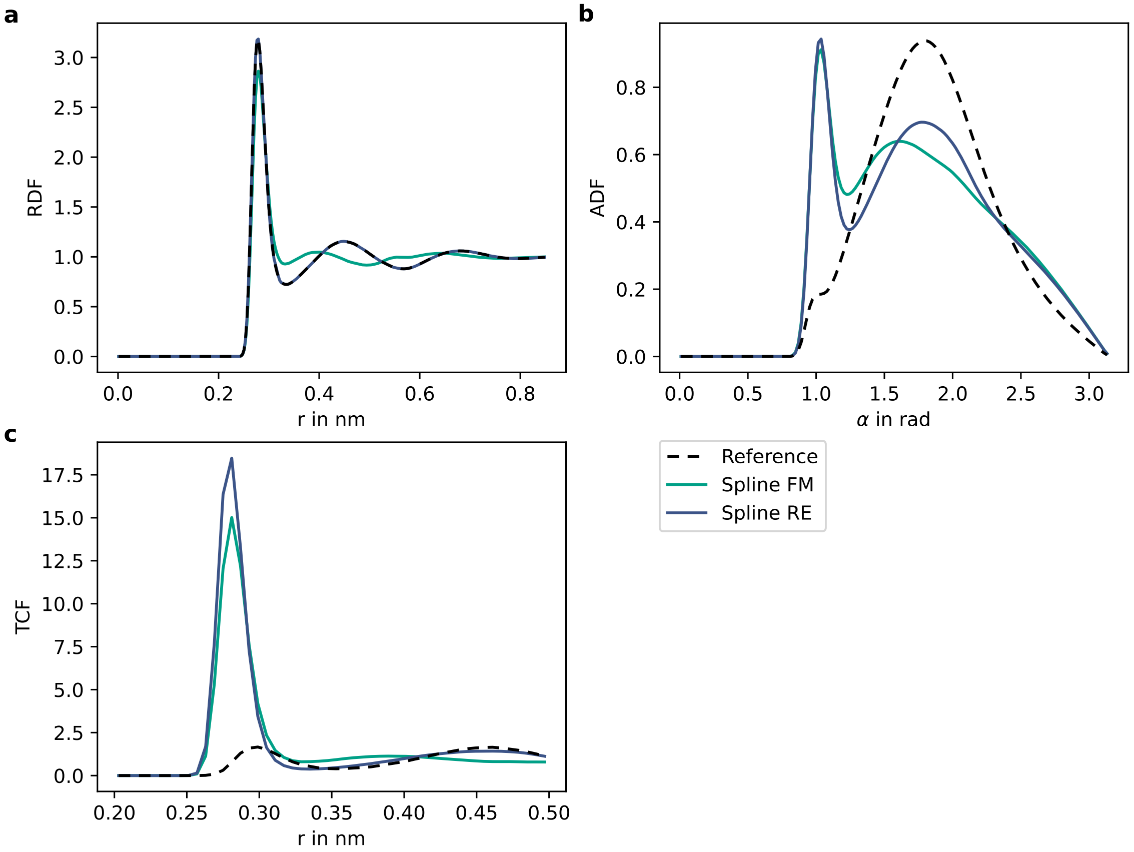


Figure 3: Liquid water spline models. Resulting (**a**) radial (RDF) and (**b**) angular distribution function (ADF) [5] as well as (**c**) equilateral triplet correlation function (TCF) [9, 10] of 2-body cubic spline models trained via force matching (FM) and relative entropy (RE) minimization compared to the atomistic reference.

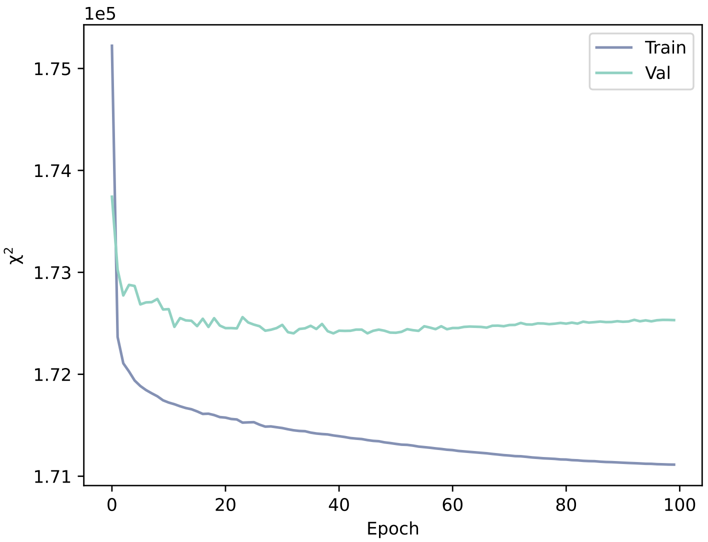


Figure 4: Alanine dipeptide loss curves. Per-epoch training and validation loss $\chi^2$ for force matching training of the alanine dipeptide model.

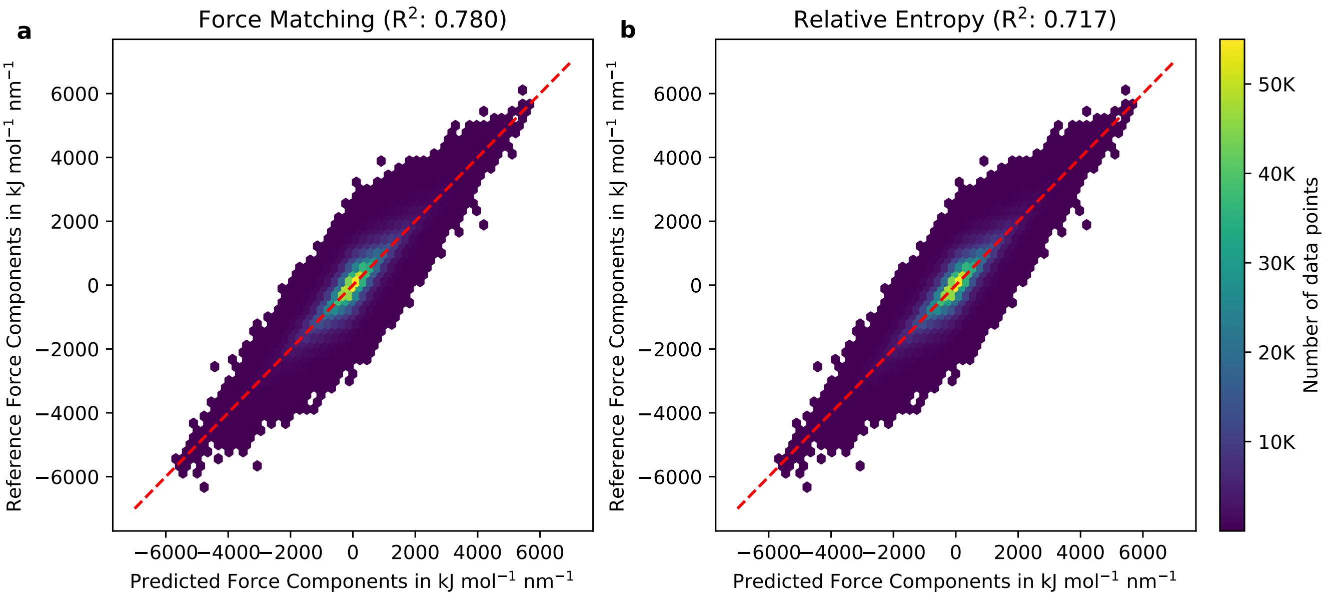


Figure 5: Alanin dipeptide force predictions on test data. Each data point corresponds to a predicted force component for a coarse-grained particle in the test data set compared to its atomistic reference for models trained via (**a**) force matching and (**b**) relative entropy minimization.

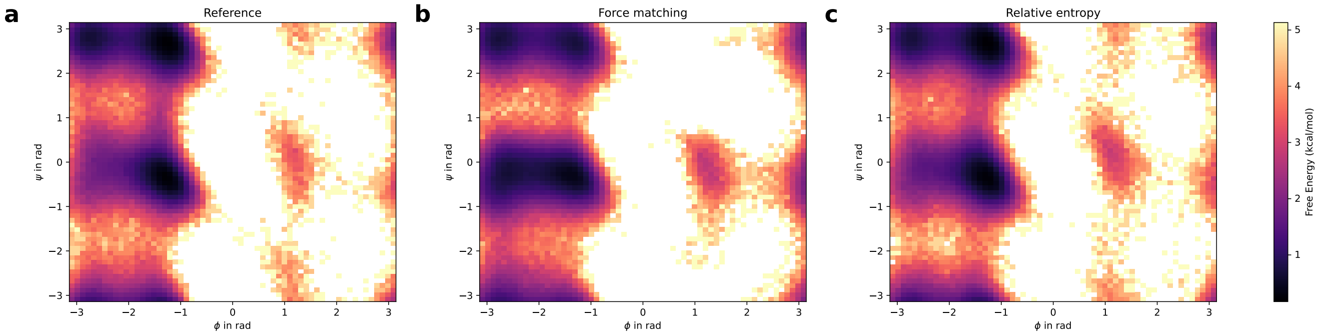


Figure 6: Free energy surface. Resulting free energy surface of the dihedral angles $\phi$ and $\psi$ from (**a**) the AT reference simulation and from the CG models trained via (**b**) force matching and (**c**) relative entropy minimization.

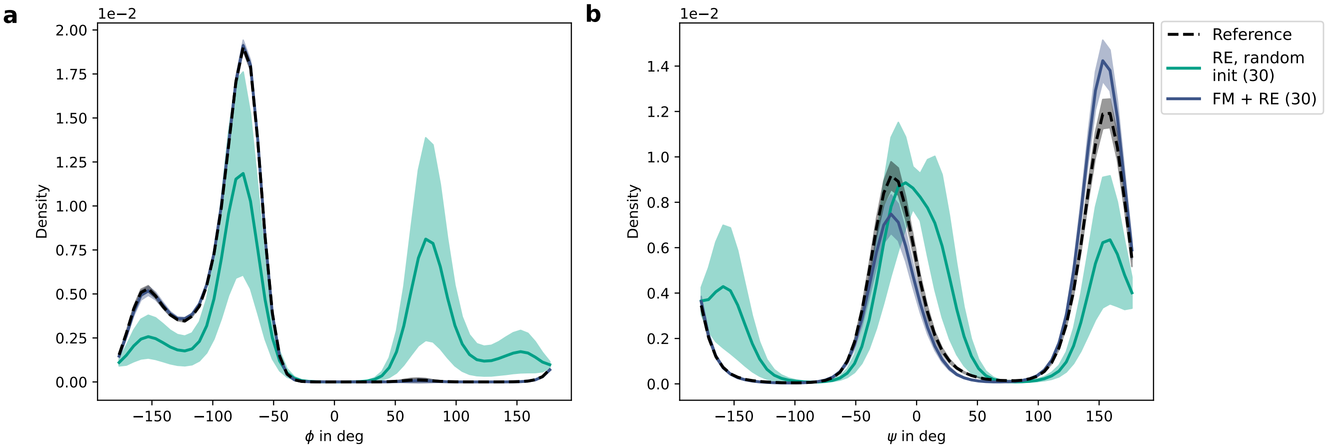


Figure 7: Dihedral angle density. Distribution of dihedral angles (**a**) $\phi$ and (**b**) $\psi$ as predicted from CG models trained via 30 relative entropy (RE) updates, compared to the atomistic reference. One model is initialized with random parameters and the other one is initialized to the parameters obtained from force matching (FM) pre-training. The mean and standard deviation (shaded area) are computed from 50 trajectories of 100 ns length.

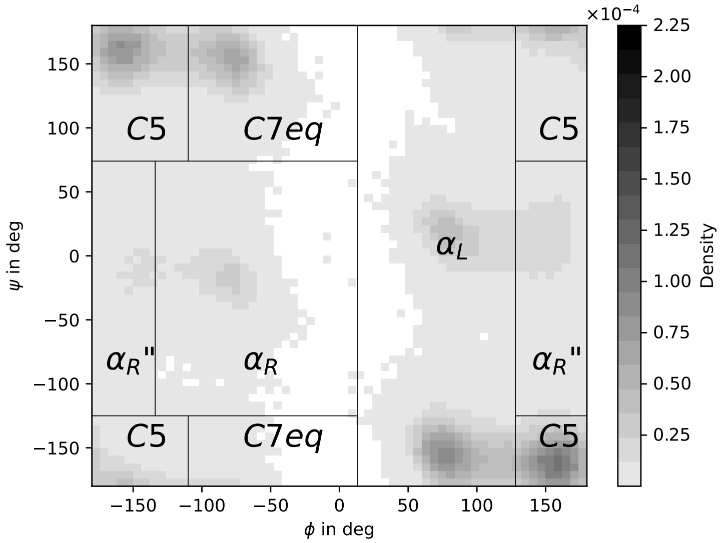


Figure 8: Force matching bond prior Ramachandran diagram. Resulting density histogram of the dihedral angles $\phi$ and $\psi$ of a single 100 ns trajectory as predicted from the CG model trained via force matching with only bonds as prior potential. This specific trajectory was selected to showcase the undesired behaviour in the $\alpha_L$ region.

## Supplementary References


[1] Kingma, D. P. & Ba, J. L. Adam: A method for stochastic optimization. In *3rd International Conference on Learning Representations, ICLR* (2015).

[2] Schoenholz, S. S. & Cubuk, E. D. JAX, M.D.: A Framework for Differentiable Physics. In *Advances in Neural Information Processing Systems*, vol. 33 (2020).

[3] Thompson, A. P. *et al.* Lammps-a flexible simulation tool for particle-based materials modeling at the atomic, meso, and continuum scales. *Comput. Phys. Commun.* **271**, 108171 (2022).

[4] Martyna, G. J., Klein, M. L. & Tuckerman, M. Nosé-Hoover chains: The canonical ensemble via continuous dynamics. *J. Chem. Phys.* **97**, 2635–2643 (1992).

[5] Soper, A. K. & Benmore, C. J. Quantum differences between heavy and light water. *Phys. Rev. Lett.* **101**, 065502 (2008).

[6] Abraham, M. J. *et al.* Gromacs: High performance molecular simulations through multi-level parallelism from laptops to supercomputers. *SoftwareX* **1**, 19–25 (2015).

[7] Duan, C., Y.and Wu *et al.* A point-charge force field for molecular mechanics simulations of proteins based on condensed-phase quantum mechanical calculations. *J. Comput. Chem.* **24**, 1999–2012 (2003).

[8] Bussi, G., Donadio, D. & Parrinello, M. Canonical sampling through velocity rescaling. *J. Chem. Phys.* **126**, 014101 (2007).

[9] Bildstein, B. & Kahl, G. Triplet correlation functions for hard-spheres: Computer simulation results. *J. Chem. Phys.* **100**, 5882 (1994).

[10] Dhabal, D., Singh, M., Wikfeldt, K. T. & Chakravarty, C. Triplet correlation functions in liquid water. *J. Chem. Phys.* **141**, 174504 (2014).
